# Supplementary material for: Axions in Cold Dark Matter and Inflation Models
Source: arXiv:1111.5281 source file (2011-11-22)
Supplement: Supplementary file 1 [file appendix.tex]

\chapter{Appendix Title}\label{appendix}
\fixchapterheading
\section*{Section Name}\label{Section Name.section}
\setcounter{thrm}{0} %% Resets theorem numbering
